# Supplementary material for: How does Early Stopping Help Generalization against Label Noise?
Source: arXiv:1911.08059 source file (2020-09-08)

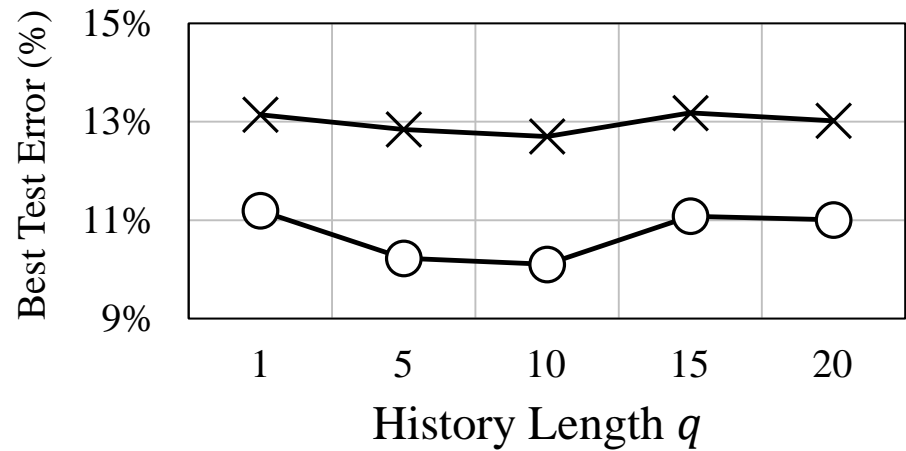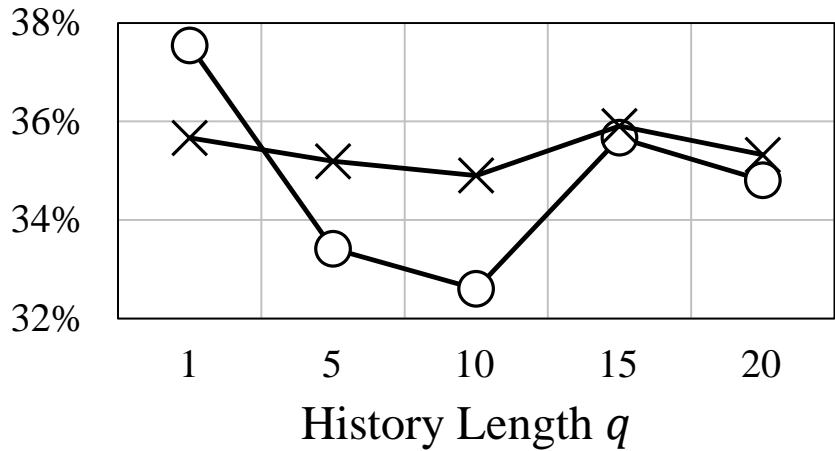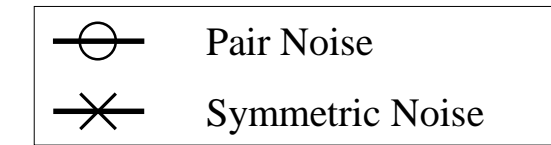

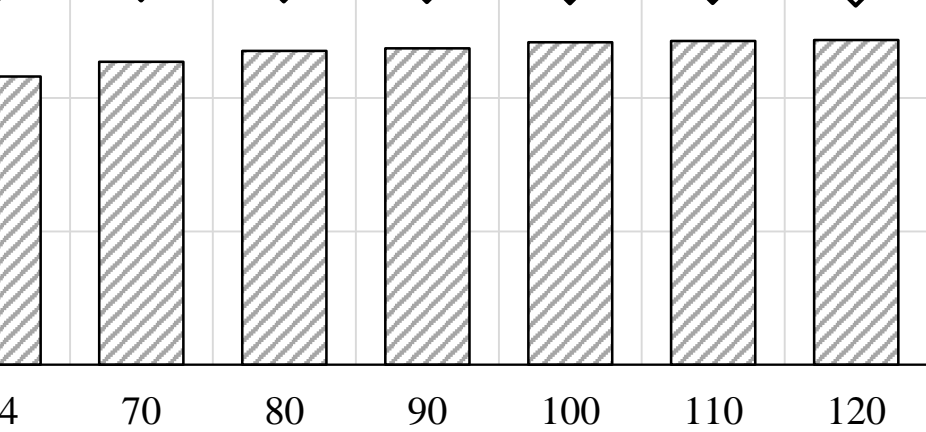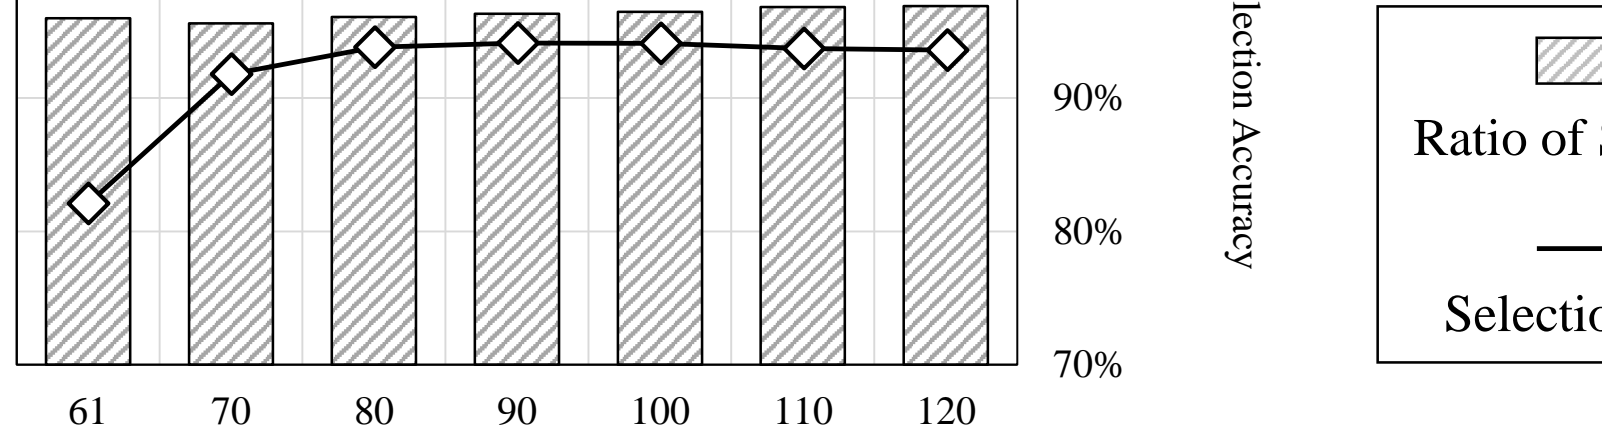

Supplement: Supplementary file 1 [file gridsearch.pdf]
