# Supplementary material for: How does Early Stopping Help Generalization against Label Noise?
Source: arXiv:1911.08059 source file (2020-09-08)

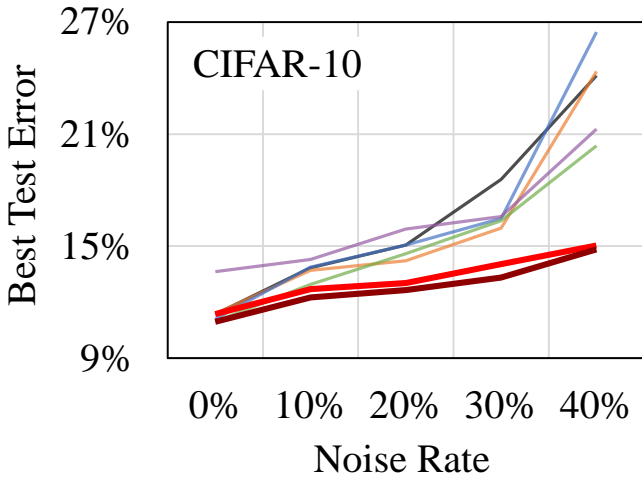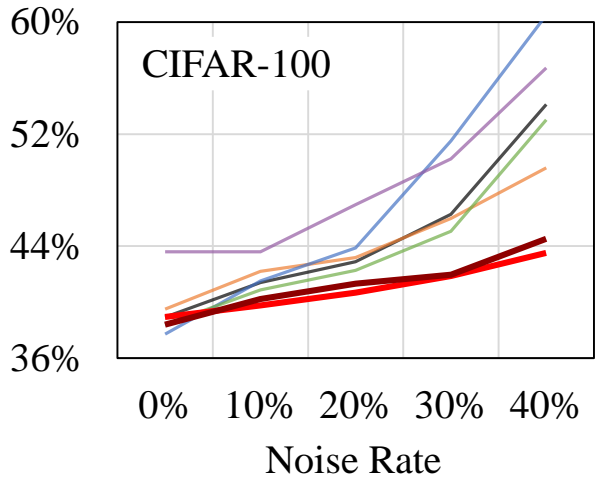

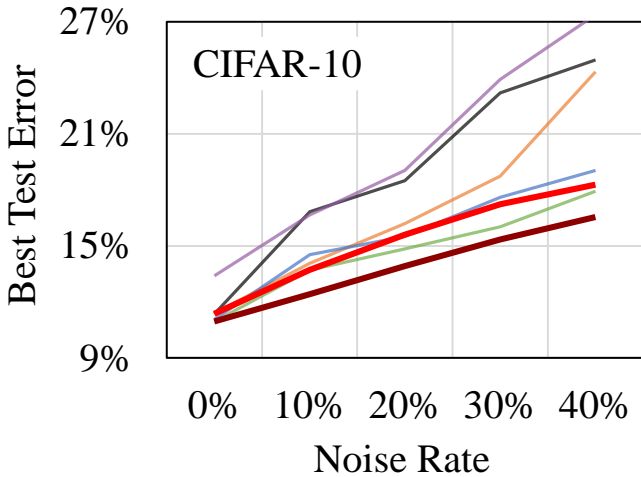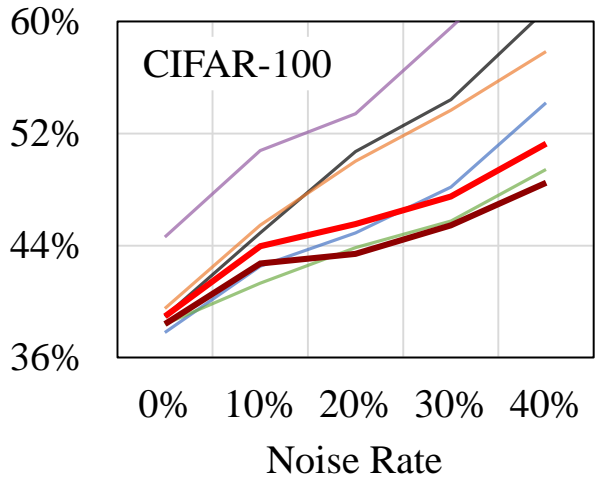

Best Test Error

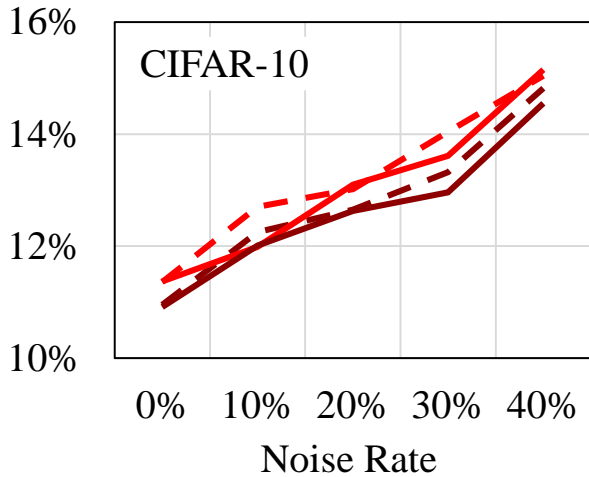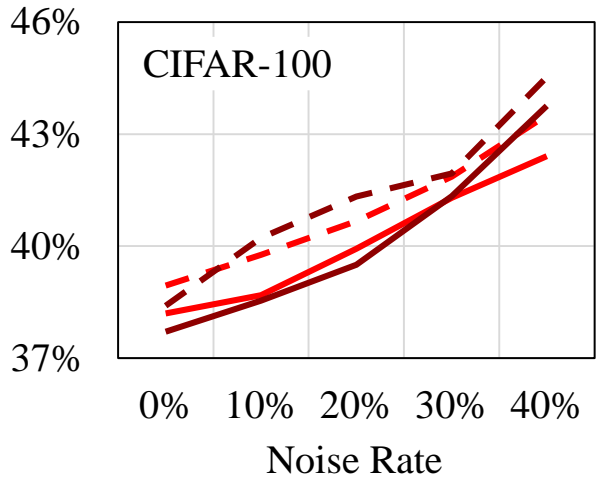

Best Test Error

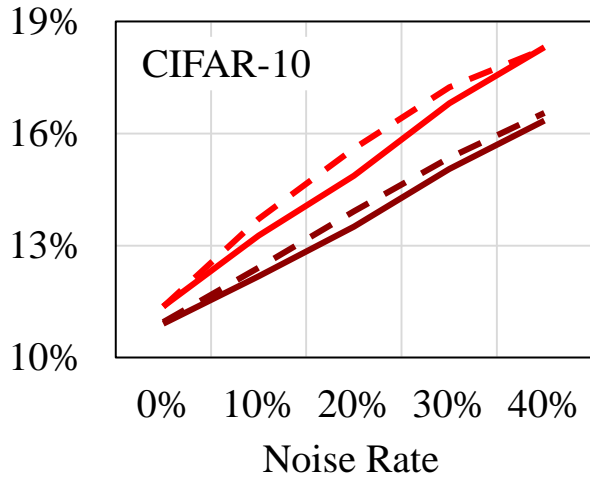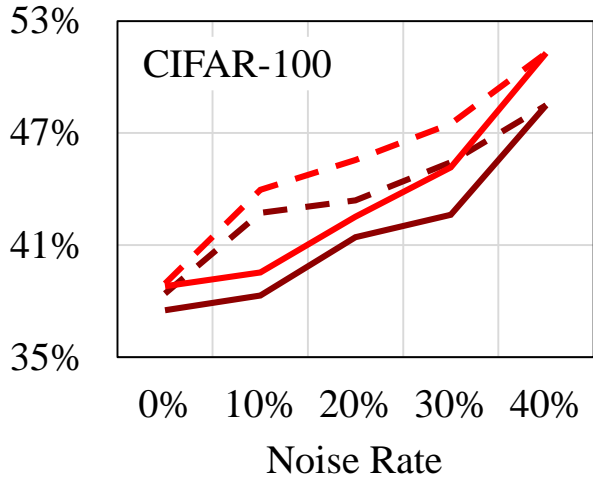

Supplement: Supplementary file 4 [file synthetic_noise_type.pdf]
